# Supplementary material for: Semantic-Anchored Evidential Fusion for Domain-Robust Whole-Slide Survival Analysis
Source: arXiv:2606.19966 source file (2026-09-22)
Supplement: Supplementary file 1 [file 6_appendix.tex]

\subsection{Semantic Anchor Generation via Slide-Level VQA}
\label{sec:anchor_gen_detail}

\subsubsection{Slide-Level Vision-Language Model}

To generate semantic anchors for each WSI, we employ ALPaCA~\cite{gao2025alpaca}, a slide-level large vision-language model (LVLM) purpose-built for WSI question answering. ALPaCA couples the CONCH~\cite{lu2024avisionlanguage} vision encoder with Llama3.1-8B~\cite{touvron2023llama}. Given a WSI, tissue regions are first detected and tessellated into patches at three magnification levels (40$\times$, 20$\times$, and 10$\times$), each resized to $224 \times 224$ pixels. A frozen CONCH encoder then extracts a 512-dimensional embedding per patch, yielding hierarchical patch representations across all three scales.

These patch embeddings are compressed into slide-level tokens through ALPaCA's hybrid adaptor, which integrates two complementary components: (1)~a Gaussian Mixture Model (GMM)-based prototyping module that distills patch embeddings into a set of 1025-dimensional morphological prototypes, capturing dominant global tissue patterns; and (2)~a LongFormer-based vision-text interaction module that refines patch embeddings conditioned on the input question, producing question-aware local visual representations of 512 dimensions. Both modules generate 32, 16, and 8 tokens for 40$\times$, 20$\times$, and 10$\times$ magnifications, respectively. After a resampler layer projects them to 4096 dimensions, the tokens from the two modules are combined additively and concatenated with text tokens as input to Llama3.1 for answer generation. ALPaCA was trained on over 35,000 WSIs with curated descriptions and 341,051 question-answer pairs from TCGA and GTEx, achieving over 90\% accuracy on closed-ended slide-level questions.

\subsubsection{Template-Based Question Design}

We design a fixed set of 12 template-based multiple-choice questions that target clinically relevant prognostic attributes. These questions were generated with GPT-5.2. Each question offers four categorical options (A--D), where the last option is always ``not assessable in this slide'', providing a built-in abstention mechanism that mitigates hallucination risk. The complete question template is presented in~\cref{tab:vqa_template}. Notably, the text of each option is a self-contained descriptive phrase that combines the prognostic attribute with its categorical level (e.g., ``Mild cellular atypia'', ``High mitotic activity'', ``No vascular or lymphatic invasion''), so that every answer constitutes a semantically complete clinical statement rather than an isolated modifier.

For each WSI, we query ALPaCA with all 12 questions and collect the predicted categorical answers. Because the responses follow a fixed template with bounded categories, the resulting semantic descriptions occupy a controlled and interpretable feature space. We encode the 12 answers into a semantic feature vector by mapping each categorical response to a numerical index and concatenating them, yielding a compact 12-dimensional descriptor that captures high-level prognostic semantics. This template-based design ensures that the semantic anchors remain consistent across centers: regardless of staining protocols or scanner differences, the same underlying pathological concept (e.g., ``high mitotic activity'' or ``no vascular invasion'') maps to the same discrete category, thereby providing the domain-invariant anchoring that motivates our framework.

% ===================== TABLE =====================
\begin{table*}[t]
\centering
\caption{Template-based VQA questions for semantic anchor generation. Each question targets a specific prognostic attribute and provides four categorical options (A--D). Every option is a self-contained phrase that combines the prognostic attribute with its categorical level, ensuring each answer constitutes a complete clinical description. Option~D denotes that the region relevant to the queried attribute is not assessable in the slide (e.g., “Mitotic activity not assessable in this slide”).}
\label{tab:vqa_template}
\resizebox{\textwidth}{!}{%
\begin{tabular}{clllll}
\toprule
\textbf{ID} & \textbf{Prognostic Attribute} & \textbf{Option A} & \textbf{Option B} & \textbf{Option C} & \textbf{Option D} \\
\midrule
Q1  & Cellular atypia              & Mild cellular atypia              & Moderate cellular atypia              & Severe cellular atypia              & Not assessable \\
Q2  & Nuclear atypia               & Mild nuclear atypia               & Moderate nuclear atypia               & Severe nuclear atypia               & Not assessable \\
Q3  & Mitotic activity             & Low mitotic activity              & Moderate mitotic activity             & High mitotic activity               & Not assessable \\
Q4  & Tumor arrangement            & Solid tumor arrangement           & Mixed tumor arrangement               & Papillary/glandular arrangement     & Not assessable \\
Q5  & Tumor infiltration           & Minimal tumor infiltration        & Moderate tumor infiltration           & Deep tumor infiltration             & Not assessable \\
Q6  & Vascular/lymphatic invasion  & No vascular/lymphatic invasion    & Possible vascular/lymphatic invasion  & Definite vascular/lymphatic invasion & Not assessable \\
Q7  & Tumor necrosis               & No tumor necrosis                 & Focal tumor necrosis                  & Extensive tumor necrosis            & Not assessable \\
Q8  & Perineural invasion          & No perineural invasion            & Possible perineural invasion          & Definite perineural invasion        & Not assessable \\
Q9  & Fibrous response             & Minimal fibrous response          & Moderate fibrous response             & Dense fibrous response              & Not assessable \\
Q10 & Tumor margin clarity         & Well-defined tumor margin         & Partially infiltrative tumor margin   & Poorly defined tumor margin         & Not assessable \\
Q11 & Angiogenesis                 & Low angiogenesis                  & Moderate angiogenesis                 & High angiogenesis                   & Not assessable \\
Q12 & Carcinoma in situ            & No carcinoma in situ              & Possible carcinoma in situ            & Definite carcinoma in situ          & Not assessable \\
\bottomrule
\end{tabular}%
}
\end{table*}


\subsection{Implementation Details}
\label{sec:impl_details}

For all baseline methods, we strictly follow the training configurations reported in their original publications, including learning rate, optimizer, batch size, and augmentation strategies, to ensure a fair comparison.

For our proposed SAEFS, we fix the semantic alignment weight $\lambda = 0.5$ and the temperature coefficient $\alpha = 1.0$ throughout all experiments. Hyperparameters were selected via five-fold cross-validation on the source domain and kept constant across all target domains without further tuning. All remaining training settings inherit from the corresponding baseline to isolate the effect of our method. This protocol ensures that any observed improvement is attributable to the semantic anchor–guided feature shifting mechanism rather than to hyperparameter optimization on the target data.

\subsection{Justification of Adaptive Evidence Mixing and Cautious Belief Fusion}

We further clarify the design rationale of the adaptive mixing and cautious fusion mechanisms used in SAEFS.
The two visual branches capture complementary aspects of WSI information.
The WSI-only branch aggregates global morphological patterns from the entire slide and therefore preserves rich contextual cues.
However, because it operates directly on raw visual features, it may also encode domain-specific artifacts such as staining variation or scanner characteristics.
In contrast, the text-guided branch focuses on regions aligned with semantic anchors derived from VQA, encouraging the model to emphasize prognostically relevant structures and clinically meaningful patterns.
While this semantic guidance improves robustness to domain shift, it may also suppress useful contextual signals outside the queried semantic scope.
Consequently, neither branch is universally optimal across all cases or domains.
Adaptive mixing therefore allows the model to balance these two visual sources, enabling flexible integration of holistic visual context and semantically guided evidence.

For multimodal fusion, the semantic and visual signals are inherently correlated because the semantic anchors are derived from the same WSI.
Naively combining them may amplify shared signals and lead to overconfident predictions.
To address this issue, SAEFS adopts cautious belief fusion, which is specifically designed for combining dependent evidence sources and preserves uncertainty when modalities disagree.
This conservative integration strategy improves the reliability of survival predictions under cross-center domain shift.

\subsection{Relationship Between Domain Shift and Performance Gain.}
The t-SNE visualization in \cref{fig:tsne_7cohort} reveals substantial distribution shifts across cohorts. 
In particular, LUAD slides from TCGA, CPTAC, and NLST form clearly separated clusters, indicating a pronounced domain gap between training and external datasets. 
In contrast, the KIRC cohorts exhibit relatively smaller distribution discrepancies.

Importantly, the performance improvements of SAEFS correlate with the severity of this visual domain shift. Compared to the average baseline C-index, SAEFS achieves a gain of +0.110 on NLST-LUAD, where the inter-cohort distribution gap is substantial. In contrast, on CPTAC-KIRC, where the cohort distributions are more overlapping, the gain is a more modest +0.060. These results suggest that SAEFS is particularly effective under severe domain shift, where purely visual MIL models tend to degrade most significantly.

This behavior supports our hypothesis that semantic anchors capture higher-level pathological concepts that remain more stable across institutions, enabling more robust cross-center survival prediction.

\begin{figure}[t]
  \centering
  \includegraphics[width=\linewidth]{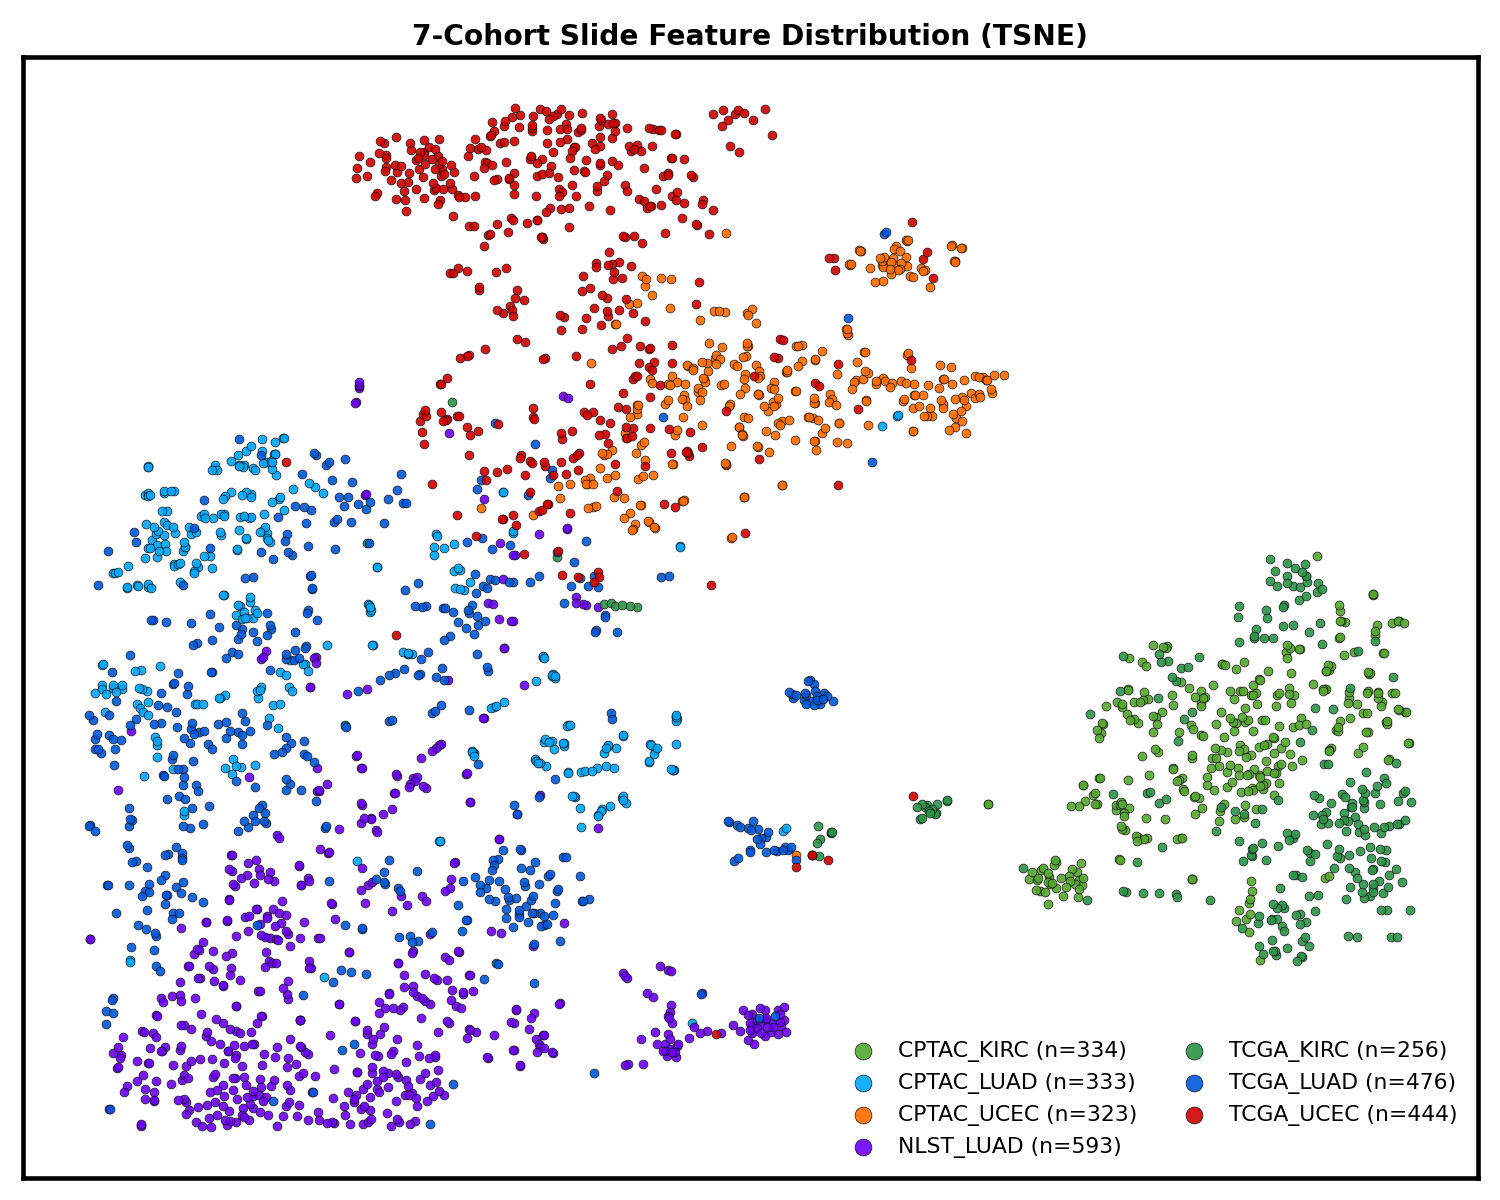}
  \caption{7-cohort slide feature distribution visualized by t-SNE.}
  \label{fig:tsne_7cohort}
\end{figure}
